# Supplementary material for: Modulational instability of Geodesic-Acoustic-Mode packets
Source: arXiv:2406.01243 source file (2024-09-30)

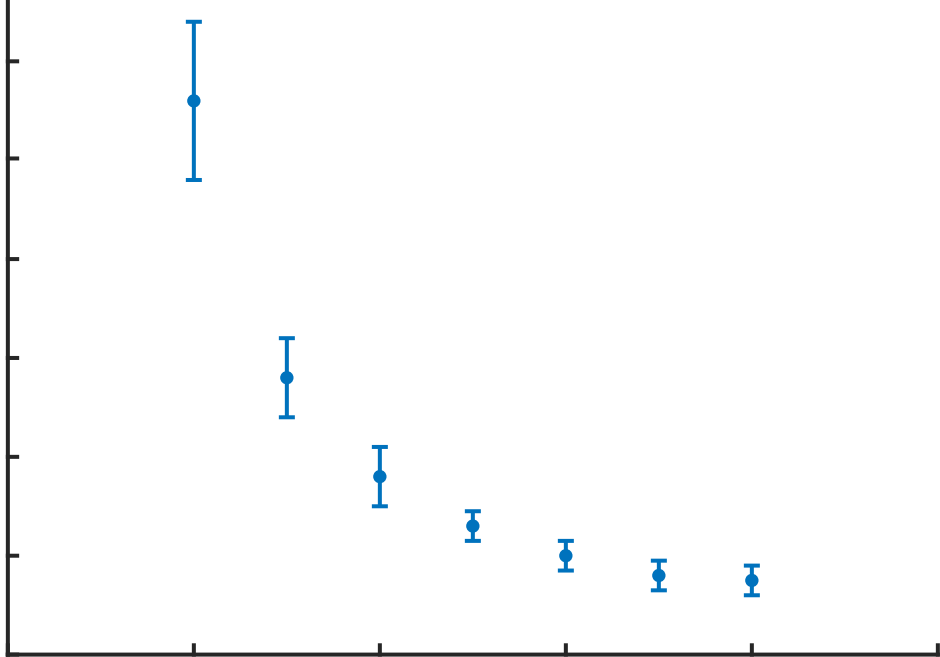

Supplement: Supplementary file 1 [file alpha-NL-vs-r0-result-31-05-23.pdf]
