# Supplementary material for: Modulational instability of Geodesic-Acoustic-Mode packets
Source: arXiv:2406.01243 source file (2024-09-30)
Supplement: Supplementary file 2 [file alpha-NL-vs-rhoi-amin-result-15-05-23.pdf]

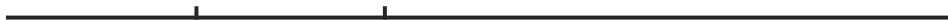

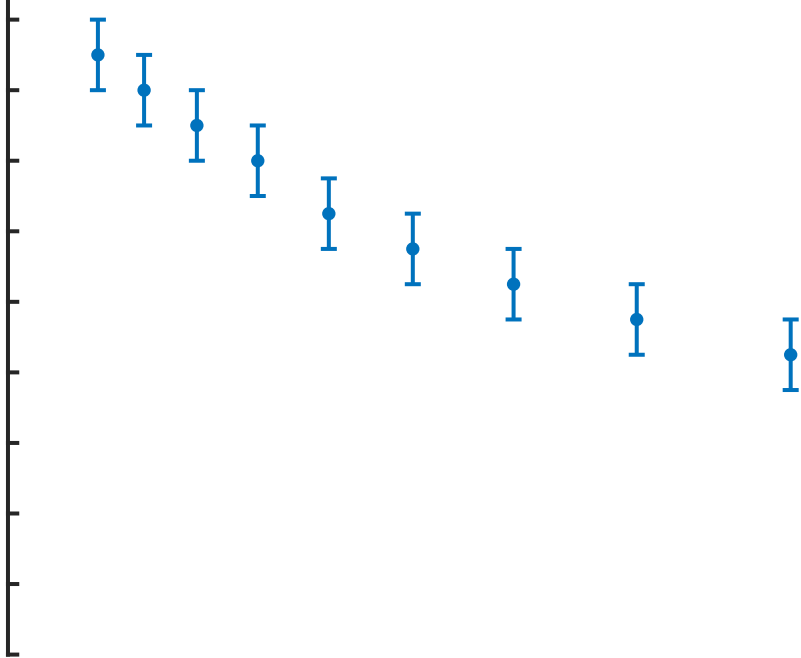

|

|
